# Supplementary material for: MIRTO: a registration-gated, multiverse-tested evaluation protocol for unsupervised anomaly segmentation in brain MRI
Source: arXiv:2610.02136 source file (2026-10-01)
Supplement: Supplementary file 1 [file appendix_prelim.tex]

\section{Preliminary rounds: five further methods on their native pipelines}\label{app:prelim}

Before the canonical pipeline existed, five further methods were trained and scored on their own pipelines: our earlier StRegA~\cite{chatterjee2022strega}, SCRD4AD~\cite{li2025scrd}, MAD-AD~\cite{beizaee2025madad}, IterMask3D~\cite{liang2025itermask3d} and Dinomaly2~\cite{guo2025dinomaly2}. Table~\ref{tab:native} reports them for completeness. The rows are \emph{not} comparable with each other or with any canonical table: each method is scored against its own resampled reference, on its own slice subset and with its legacy voxel volume, which are exactly the sources of error that Section~\ref{sec:R} removes, and for four of the five methods the threshold was tuned on the test cohort, so their values are optimistic upper bounds. StRegA was re-scored with a threshold fitted on the 24 validation subjects; its median volume Dice was 0.167 to 0.180 in the four T2 configurations and 0.119 to 0.132 in the four T1 configurations. These values are not comparable with the Dice of 0.642 originally reported for StRegA on BraTS T2~\cite{chatterjee2022strega}, which was obtained with a different preprocessing, reference and threshold protocol. Thirteen further rows were excluded for documented reasons: swapped labels (StRegA D7, D8), sub-chance slice AUROC (SCRD4AD 7, 8), FAST-preprocessed inputs (seven rows), a diverged training run (MAD-AD 5) and a saturated normalisation with the threshold at the grid ceiling (Dinomaly2 B1).
\begin{table}[H]
\caption{Preliminary native five-method table (Rounds 1--2): median volume Dice and small-stratum Dice. Not comparable across rows or with the canonical tables; ``test-tuned $\tau$'' rows are optimistic upper bounds. MAD-AD cohort size is not stated in its source file.}
\label{tab:native}
\centering\scriptsize
\setlength{\tabcolsep}{4pt}
\resizebox{\textwidth}{!}{%
\begin{tabular}{@{}lllllll@{}}
\toprule
Method & Config & Test contrast & Cohort & $\tau$ provenance & Volume Dice, median [IQR] & Small-stratum Dice, median\\
\midrule
StRegA & D1 & T1 & 312 & val.\ $\tau$ (R2) & 0.126 [IQR 0.059, 0.219] & 0.000\\
StRegA & D2 & T1 & 312 & val.\ $\tau$ (R2) & 0.132 [IQR 0.071, 0.185] & 0.010\\
StRegA & D3 & T1 & 312 & val.\ $\tau$ (R2) & 0.119 [IQR 0.070, 0.180] & 0.015\\
StRegA & D4 & T2 & 312 & val.\ $\tau$ (R2) & 0.178 [IQR 0.082, 0.291] & 0.001\\
StRegA & D5 & T2 & 312 & val.\ $\tau$ (R2) & 0.180 [IQR 0.099, 0.272] & 0.014\\
StRegA & D6 & T2 & 312 & val.\ $\tau$ (R2) & 0.175 [IQR 0.102, 0.254] & 0.020\\
StRegA & D9 & T1 & 312 & val.\ $\tau$ (R2) & 0.122 [IQR 0.071, 0.180] & 0.016\\
StRegA & D10 & T2 & 312 & val.\ $\tau$ (R2) & 0.167 [IQR 0.102, 0.246] & 0.025\\
SCRD4AD & 1 & T1 & 312 & test-tuned $\tau$ & 0.119 & 0.017\\
SCRD4AD & 2 & T1 & 312 & test-tuned $\tau$ & 0.158 & 0.007\\
SCRD4AD & 3 & T1 & 312 & test-tuned $\tau$ & 0.174 & 0.007\\
SCRD4AD & 4 & T2 & 312 & test-tuned $\tau$ & 0.361 & 0.000\\
SCRD4AD & 5 & T2 & 312 & test-tuned $\tau$ & 0.320 & 0.000\\
SCRD4AD & 6 & T2 & 312 & test-tuned $\tau$ & 0.207 & 0.001\\
SCRD4AD & 9 & T1 & 312 & test-tuned $\tau$ & 0.162 & 0.011\\
SCRD4AD & 10 & T2 & 312 & test-tuned $\tau$ & 0.161 & 0.017\\
MAD-AD & 1 & T1 & not stated & test-tuned $\tau$ & 0.204 & 0.000\\
MAD-AD & 2 & T1 & not stated & test-tuned $\tau$ & 0.141 & 0.006\\
MAD-AD & 4 & T1 & not stated & test-tuned $\tau$ & 0.191 & 0.000\\
MAD-AD & 6 & T2 & not stated & test-tuned $\tau$ & 0.458 & 0.000\\
MAD-AD & 7 & T2 & not stated & test-tuned $\tau$ & 0.255 & 0.000\\
MAD-AD & 9 & T1 & not stated & test-tuned $\tau$ & 0.158 & 0.004\\
MAD-AD & 10 & T2 & not stated & test-tuned $\tau$ & 0.206 & 0.000\\
MAD-AD & 11 & T1 & not stated & test-tuned $\tau$ & 0.103 & 0.003\\
MAD-AD & 12 & T2 & not stated & test-tuned $\tau$ & 0.187 & 0.000\\
IterMask3D & IXI\_all\_\_BraTS\_T2\_E199 & T2 & 346 & test-tuned $\tau$ & 0.221 & 0.000\\
IterMask3D & IXI\_all\_\_BraTS\_T2\_E199\_g05 & T2 & 346 & test-tuned $\tau$ & 0.186 & 0.009\\
IterMask3D & MOOD\_IXI\_all\_\_BraTS\_T1 & T1 & 346 & test-tuned $\tau$ & 0.000 & 0.000\\
IterMask3D & MOOD\_IXI\_all\_\_BraTS\_T1\_E499 & T1 & 346 & test-tuned $\tau$ & 0.017 & 0.000\\
IterMask3D & MOOD\_IXI\_all\_\_BraTS\_T1\_E499\_ext & T1 & 346 & test-tuned $\tau$ & 0.021 & 0.000\\
IterMask3D & MOOD\_IXI\_all\_\_BraTS\_T1\_pernorm & T1 & 346 & test-tuned $\tau$ & 0.001 & 0.000\\
IterMask3D & MOOD\_IXI\_all\_\_BraTS\_T2 & T2 & 346 & test-tuned $\tau$ & 0.071 & 0.000\\
IterMask3D & MOOD\_IXI\_all\_\_BraTS\_T2\_E499 & T2 & 346 & test-tuned $\tau$ & 0.077 & 0.000\\
IterMask3D & MOOD\_IXI\_all\_\_BraTS\_T2\_E499\_ext & T2 & 346 & test-tuned $\tau$ & 0.079 & 0.000\\
IterMask3D & MOOD\_IXI\_all\_\_BraTS\_T2\_pernorm & T2 & 346 & test-tuned $\tau$ & 0.085 & 0.000\\
Dinomaly2 & B2 & T1 & 312 & test-tuned $\tau$ & 0.068 & 0.000\\
Dinomaly2 & B3 & T1 & 312 & test-tuned $\tau$ & 0.089 & 0.000\\
Dinomaly2 & B4 & T2 & 312 & test-tuned $\tau$ & 0.313 & 0.000\\
Dinomaly2 & B5 & T2 & 312 & test-tuned $\tau$ & 0.354 & 0.000\\
Dinomaly2 & B6 & T2 & 312 & test-tuned $\tau$ & 0.321 & 0.000\\
Dinomaly2 & B7 & T1 & 312 & test-tuned $\tau$ & 0.119 & 0.000\\
Dinomaly2 & B8 & T2 & 312 & test-tuned $\tau$ & 0.375 & 0.000\\
Dinomaly2 & B9 & T1 & 312 & test-tuned $\tau$ & 0.116 & 0.000\\
Dinomaly2 & B10 & T2 & 312 & test-tuned $\tau$ & 0.372 & 0.000\\
\bottomrule
\end{tabular}}
\end{table}
A preliminary small-lesion analysis on the Round~2 native banks compared each small lesion with an equal-area local region (Table~\ref{tab:j2}). Local AUPRC was weakly above chance for REFLECT D10 and cDDPM D6 and not distinguishable from chance for UCCD D4 under pixel stratification, and cDDPM's local AUROC interval included 0.5. These banks predate the canonical pipeline, so the analysis is descriptive only.
\begin{table}[H]
\caption{Small-lesion local contrast (J2, preliminary; Round~2 native banks; chance level 0.5).}
\label{tab:j2}
\centering\scriptsize
\setlength{\tabcolsep}{3pt}
\begin{tabular}{@{}llllll@{}}
\toprule
Configuration (Round 2 banks) & Small-lesion definition & Lesions & Subjects & Local AUPRC [95 \% CI] (chance 0.5) & Local AUROC [95 \% CI]\\
\midrule
REFLECT D10 (primary) & pixel & 122 & 71 & 0.531 [0.511, 0.554] & 0.537 [0.516, 0.558]\\
REFLECT D10 (primary) & physical & 133 & 77 & 0.557 [0.533, 0.584] & 0.561 [0.538, 0.587]\\
cDDPM D6 (primary) & pixel & 100 & 62 & 0.535 [0.504, 0.567] & 0.484 [0.432, 0.536]\\
cDDPM D6 (primary) & physical & 127 & 81 & 0.584 [0.552, 0.617] & 0.538 [0.491, 0.584]\\
UCCD D4 (NOT the primary D5) & pixel & 120 & 74 & 0.509 [0.484, 0.536] & 0.495 [0.462, 0.528]\\
UCCD D4 (NOT the primary D5) & physical & 136 & 85 & 0.544 [0.514, 0.575] & 0.527 [0.493, 0.562]\\
\bottomrule
\end{tabular}
\end{table}
\paragraph{Compute.} Table~\ref{tab:compute} gives the recorded wall-clock and GPU time on Tesla V100 GPUs. Training records for UCCD and cDDPM in the cost table could not be verified and are omitted, and the REFLECT training run listed predates the D6 checkpoint, so it indicates the order of magnitude only. One inference over 24 validation volumes (UCCD D5) drew 89.9\,W on average, against the 300\,W rating of the GPU.
\begin{table}[H]
\caption{Compute from the Round~2 cost table (Tesla V100-SXM2-32GB). Dinomaly2 times were supplied from the thesis, not from accounting.}
\label{tab:compute}
\centering\scriptsize
\setlength{\tabcolsep}{4pt}
\begin{tabular}{@{}lllll@{}}
\toprule
Method & Phase & Wall clock & GPU-hours & s per volume\\
\midrule
REFLECT & train (stage 1) & 6d 17:25:53 & 484.29 & \\
REFLECT & train (stage 2) & 4d 07:31:24 & 207.05 & \\
REFLECT & inference & 03:07:18 & 3.12 & 32.5\\
AnomalyDINO & memory-bank build & 00:01:07 & 0.02 & \\
AnomalyDINO & inference & 00:15:23 & 0.26 & 2.7\\
IterMask3D & train & 09:15:03 & 18.50 & \\
IterMask3D & inference & 02:43:04 & 2.72 & 28.3\\
Dinomaly2 & train (per configuration) & 4h50m to 16h39m, scaling with training-set size, single V100 & 4.83 to 16.65 & \\
Dinomaly2 & calibration (per dataset) & ~00:15:00 & 0.25 & \\
Dinomaly2 & inference (per dataset) & ~00:15:00 & 0.25 & 2.6\\
\bottomrule
\end{tabular}
\end{table}
